# Supplementary material for: Real World Evaluation of Approaches to Research Paper Recommendation
Source: arXiv:1802.06892 source file (2018-02-19)
Supplement: Supplementary file 2 [file AppendixTemplate.tex]

% Appendix Template

\chapter{Appendix Title Here} % Main appendix title

\label{AppendixX} % Change X to a consecutive letter; for referencing this appendix elsewhere, use \ref{AppendixX}

\lhead{Appendix X. \emph{Appendix Title Here}} % Change X to a consecutive letter; this is for the header on each page - perhaps a shortened title

Write your Appendix content here.
